# Supplementary material for: Online Learning in Iterated Prisoner's Dilemma to Mimic Human Behavior
Source: arXiv:2006.06580 source file (2022-08-27)
Supplement: Supplementary file 1 [file sec_appendix.tex]

\clearpage
\appendix

\section{Reproducibility}

The codes and data to reproduce all the experimental results can be accessed in the supplementary materials.

\section{Supplementary Figures}
\label{sec:supp}

\begin{figure}[h!]
% \vspace{-1em}
\centering
\includegraphics[width=0.48\linewidth]{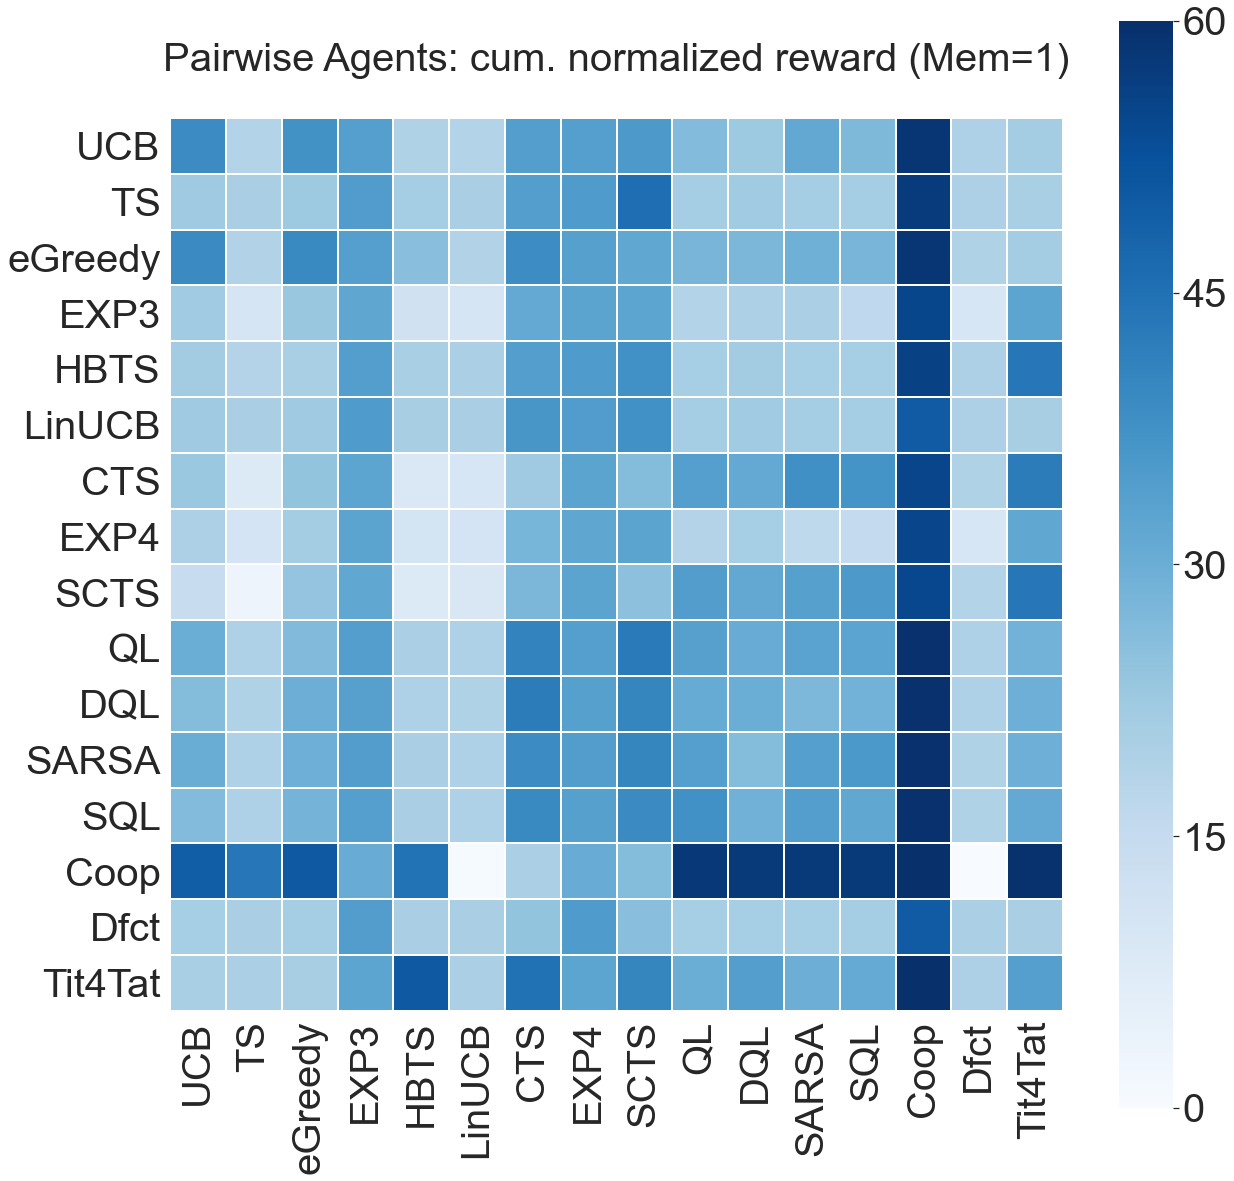}
\includegraphics[width=0.48\linewidth]{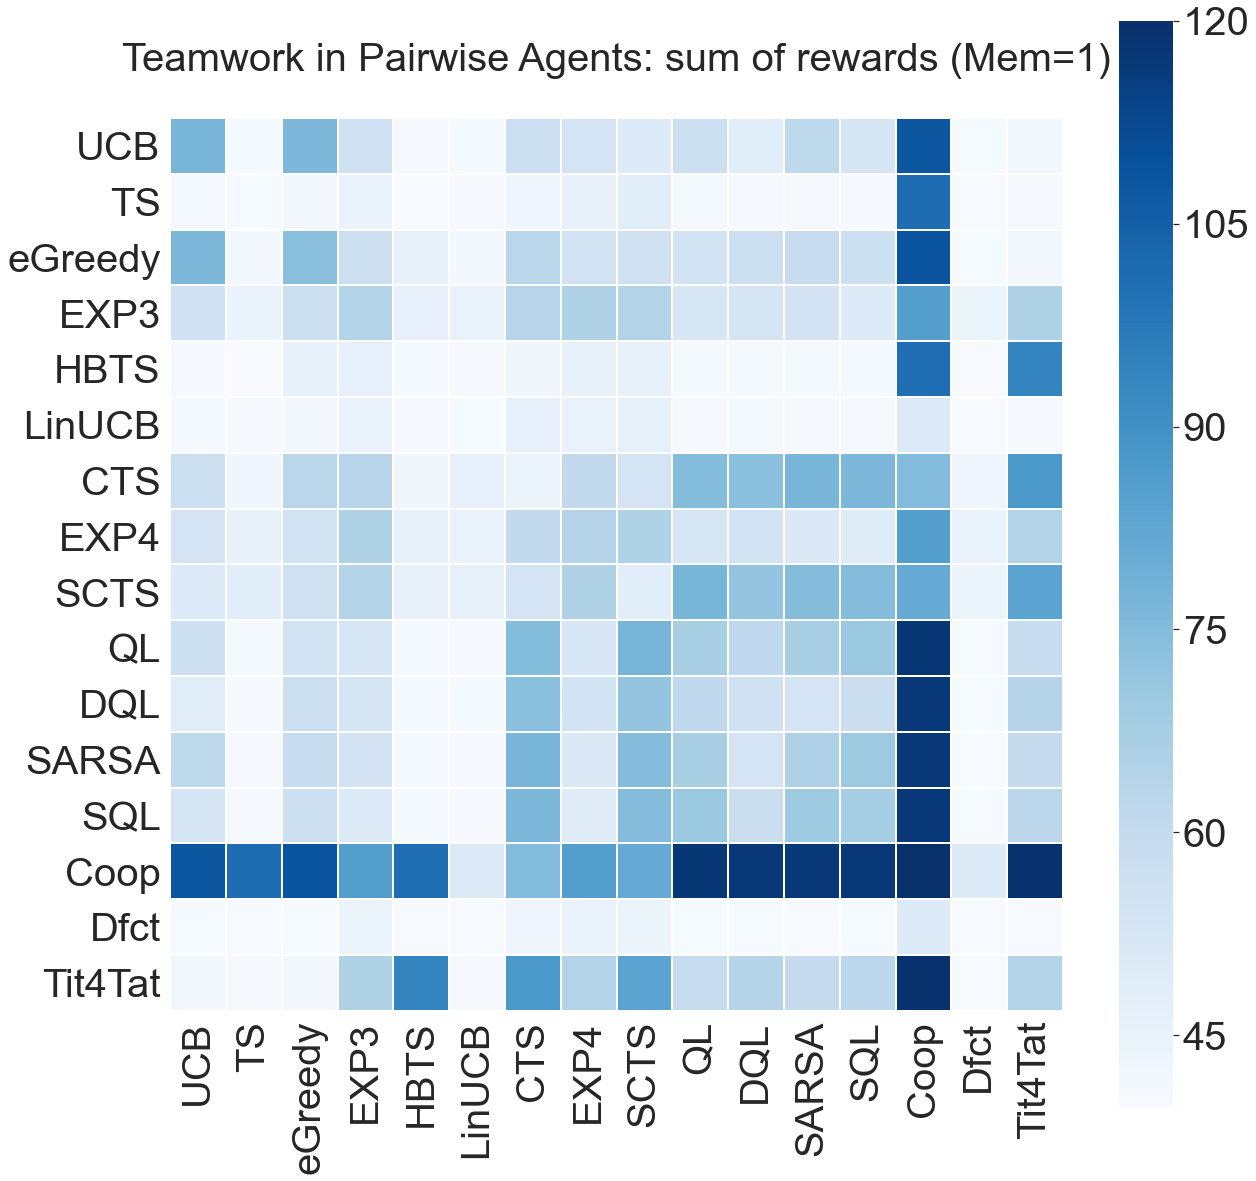}
\par\caption{Success and teamwork in two-agent tournament: individual rewards and collective rewards.}\label{fig:rp2}
\end{figure}

\begin{figure}[h!]
% \vspace{-1em}
\centering
\includegraphics[width=0.48\linewidth]{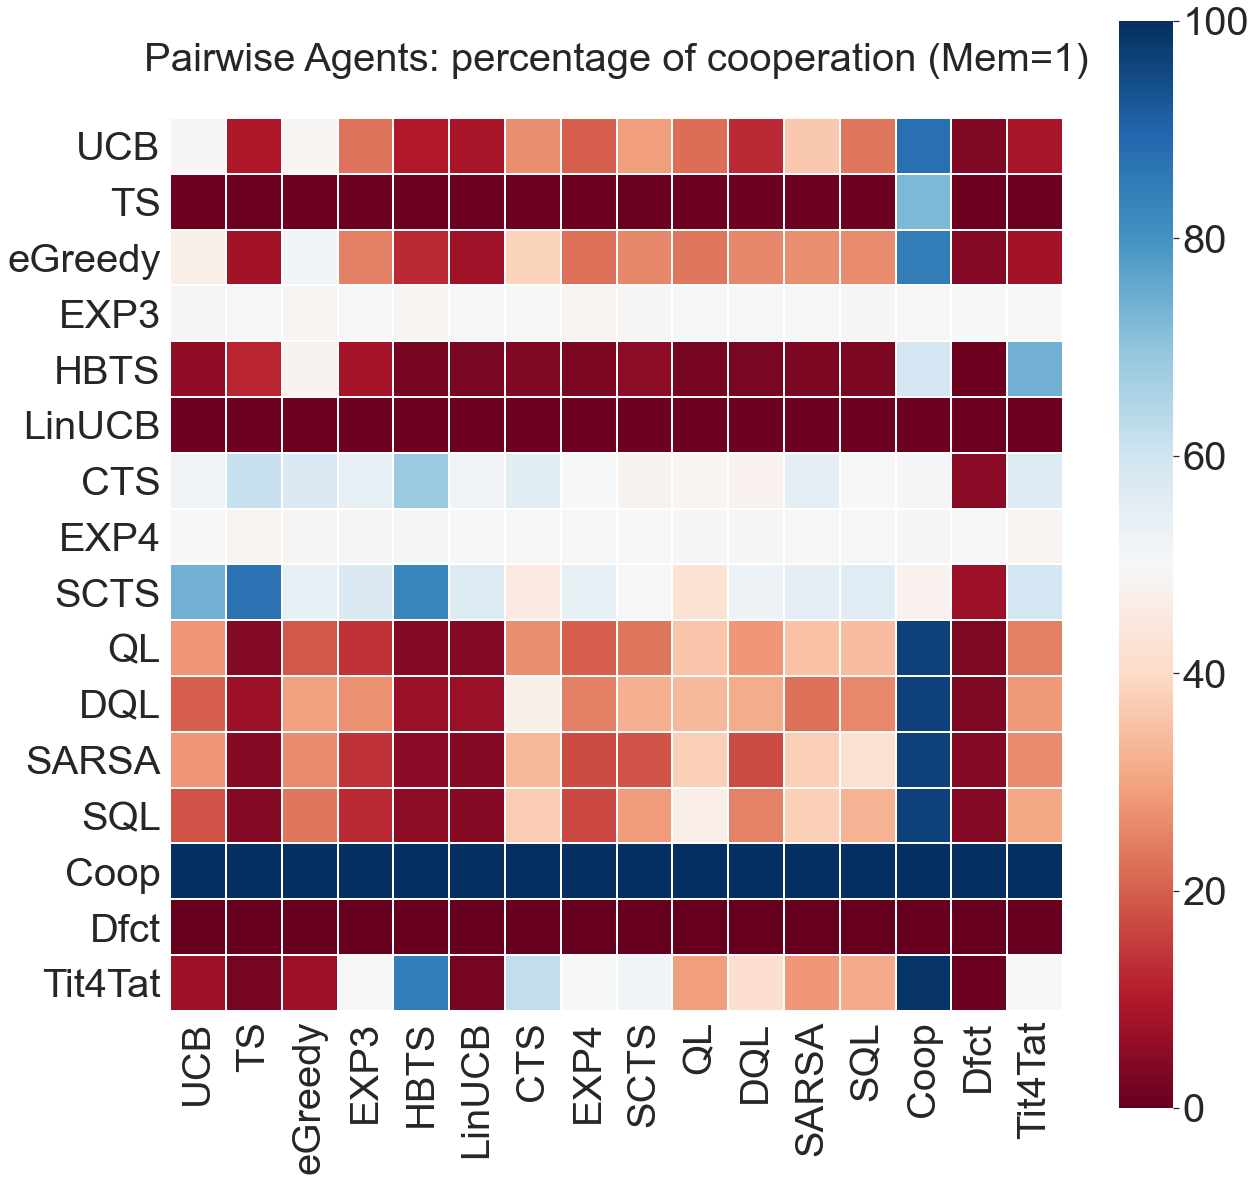}
\includegraphics[width=0.48\linewidth]{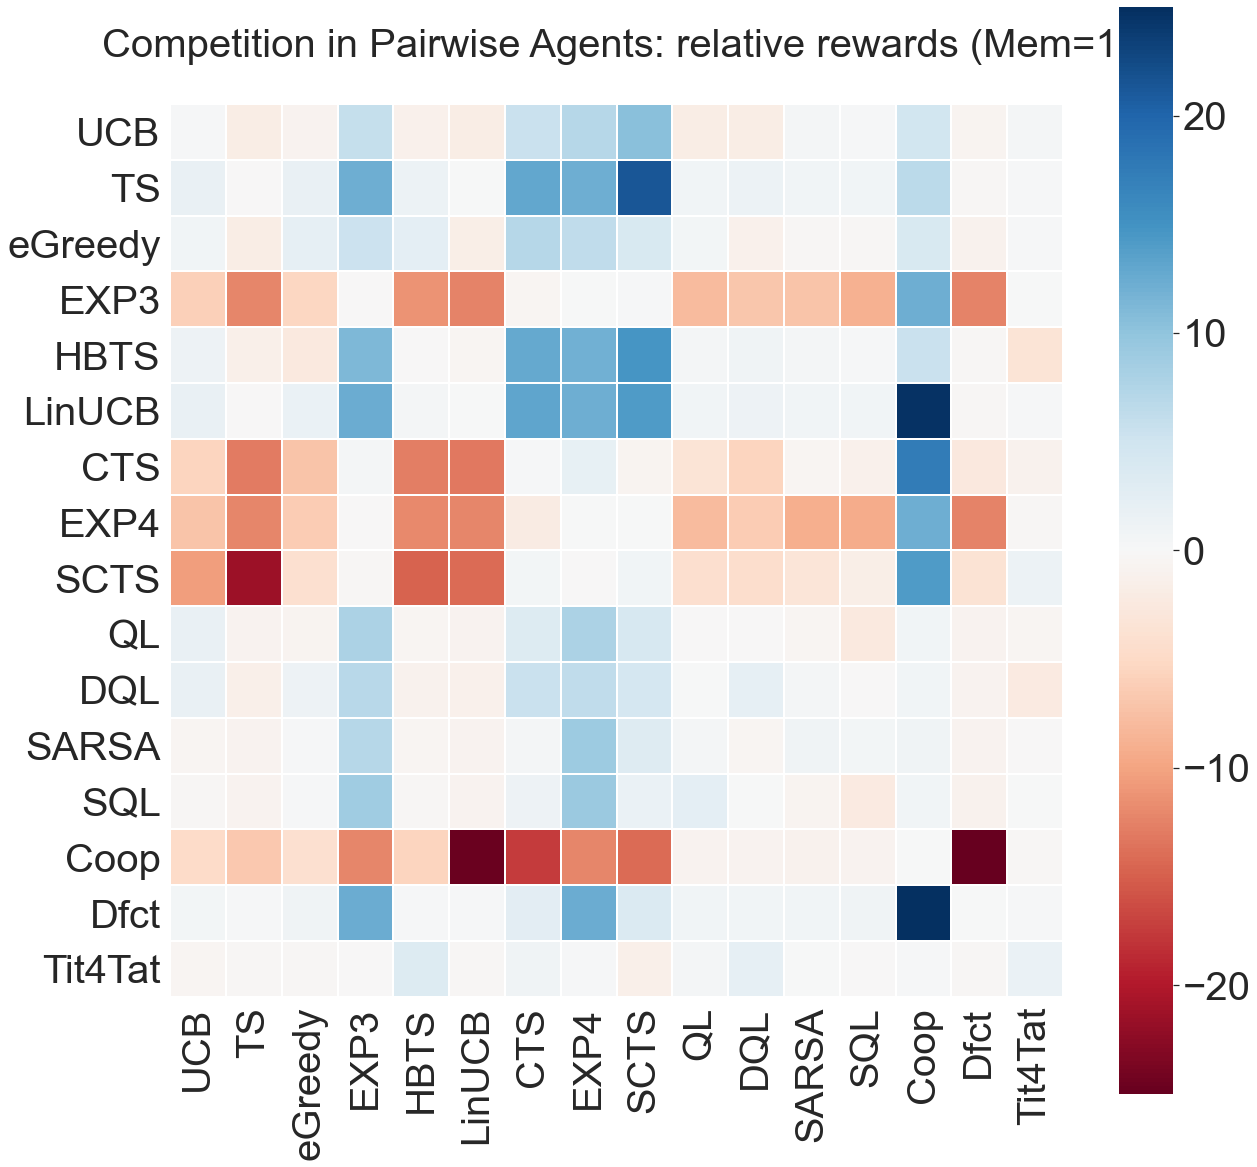}
\par\caption{Cooperation and Competition in two-agent tournament: cooperation rate, relative rewards.}\label{fig:sd2}
\end{figure}

\begin{figure}[h!]
% \vspace{-1em}
\centering
\includegraphics[width=0.24\linewidth]{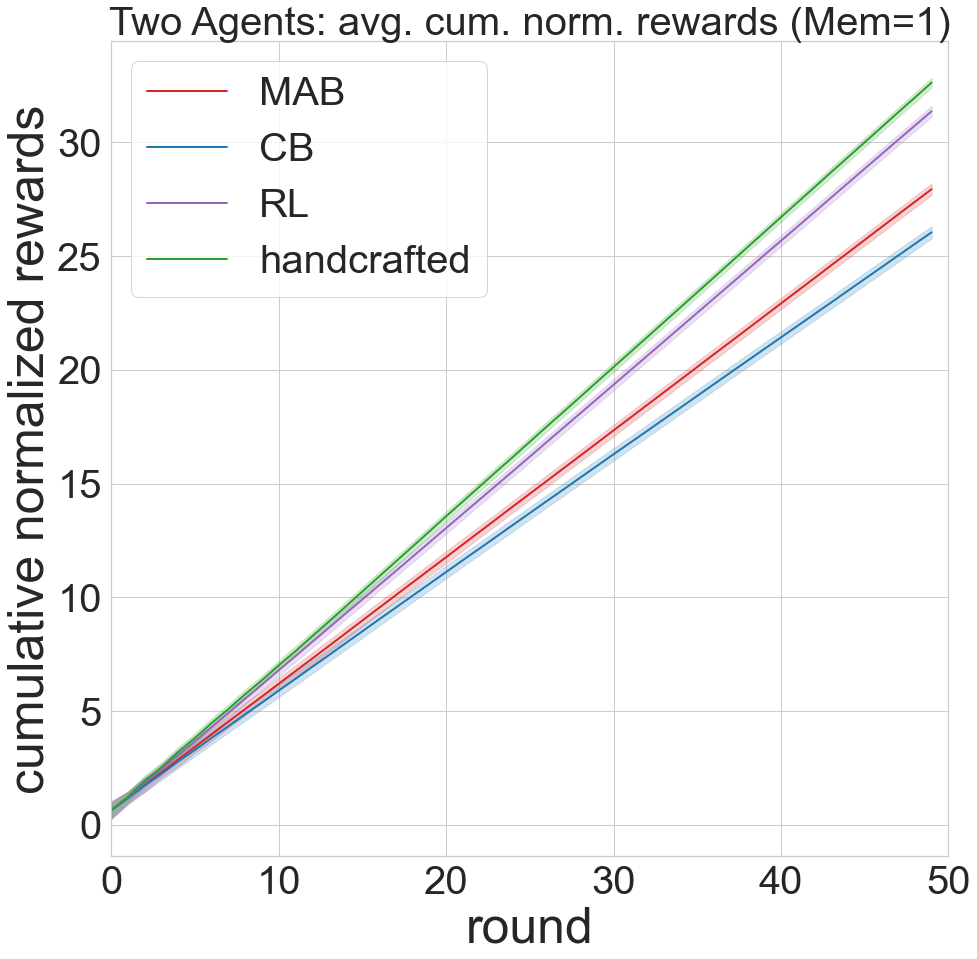}
\includegraphics[width=0.24\linewidth]{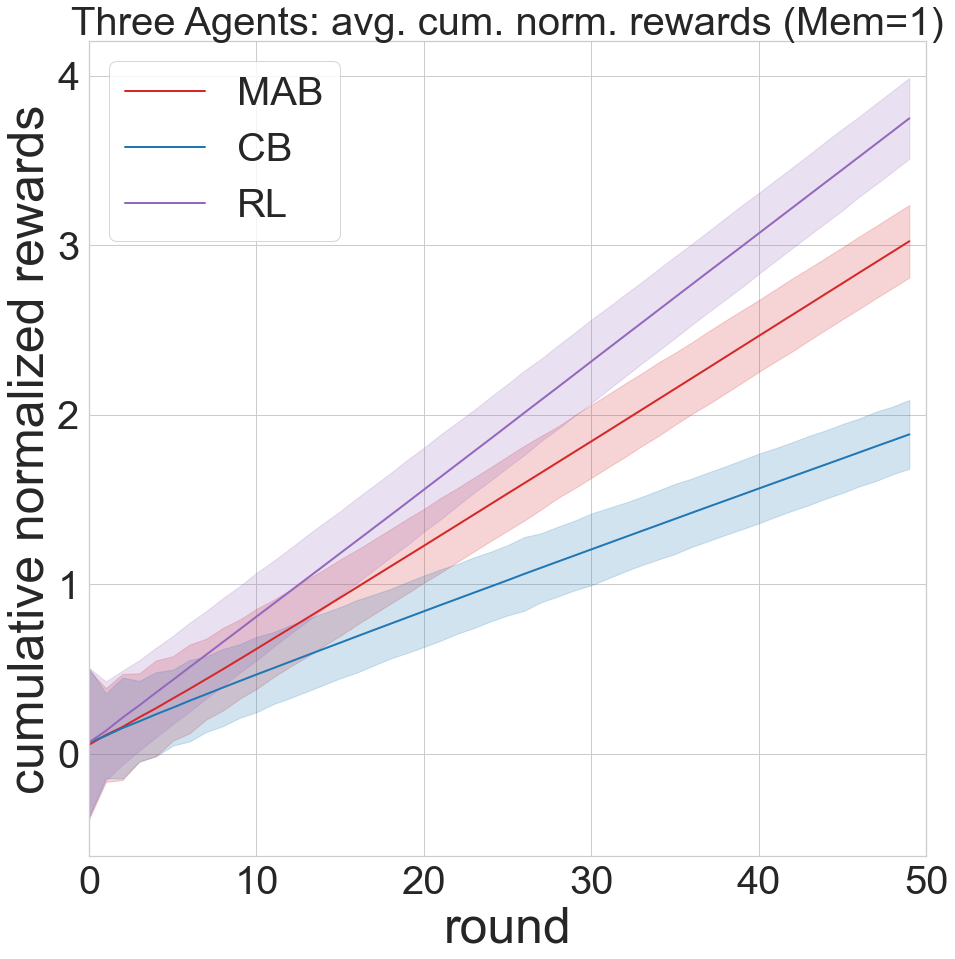}
\includegraphics[width=0.24\linewidth]{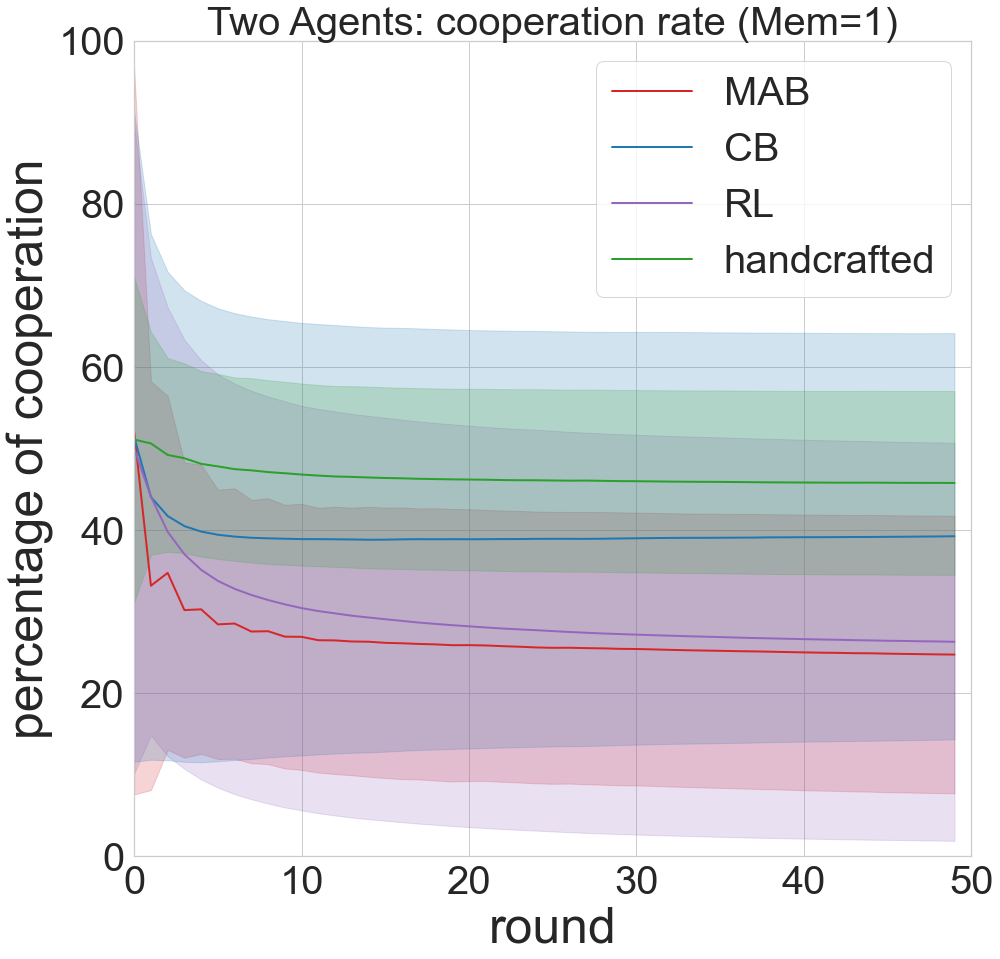}
\includegraphics[width=0.24\linewidth]{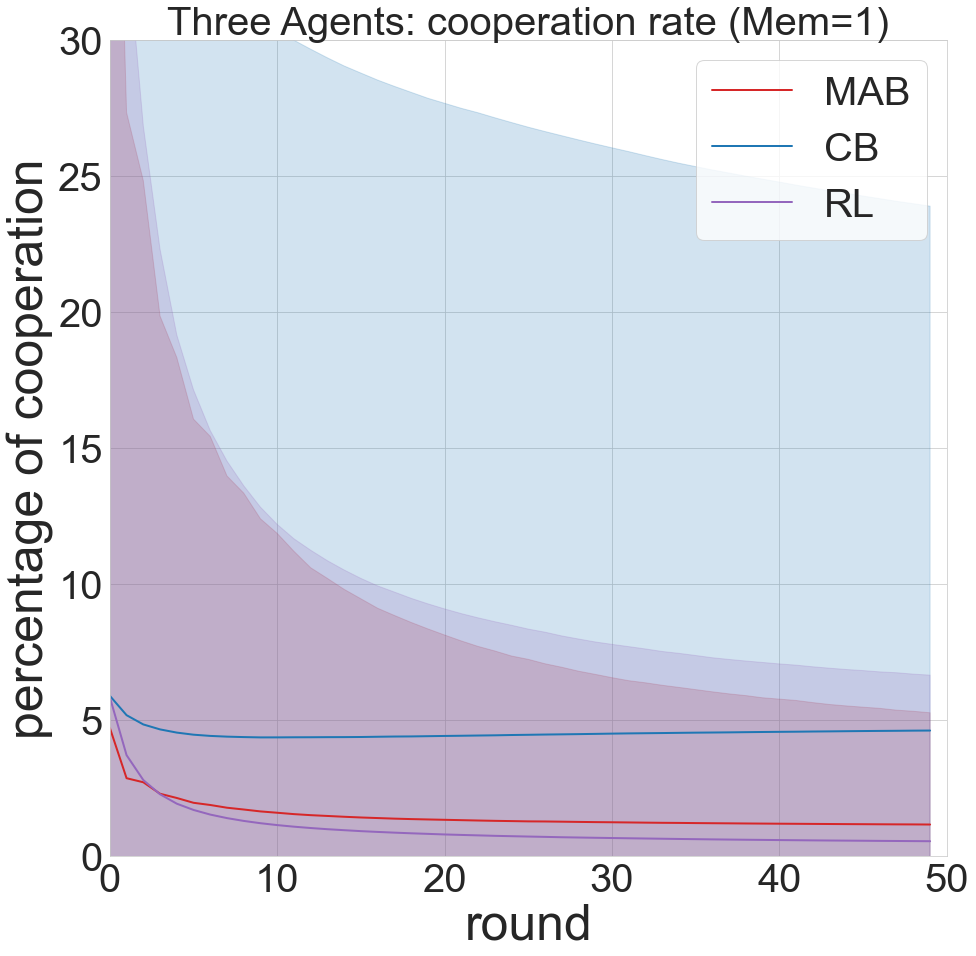}
\par\caption{Cumulative rewards and cooperation rates averaged by class in two-player and three-player setting (shown here the models trained with memory of 1 past action pairs).}\label{fig:two_three2}
\end{figure}

\begin{figure}[h!]
% \vspace{-1em}
\centering
\includegraphics[width=0.6\linewidth]{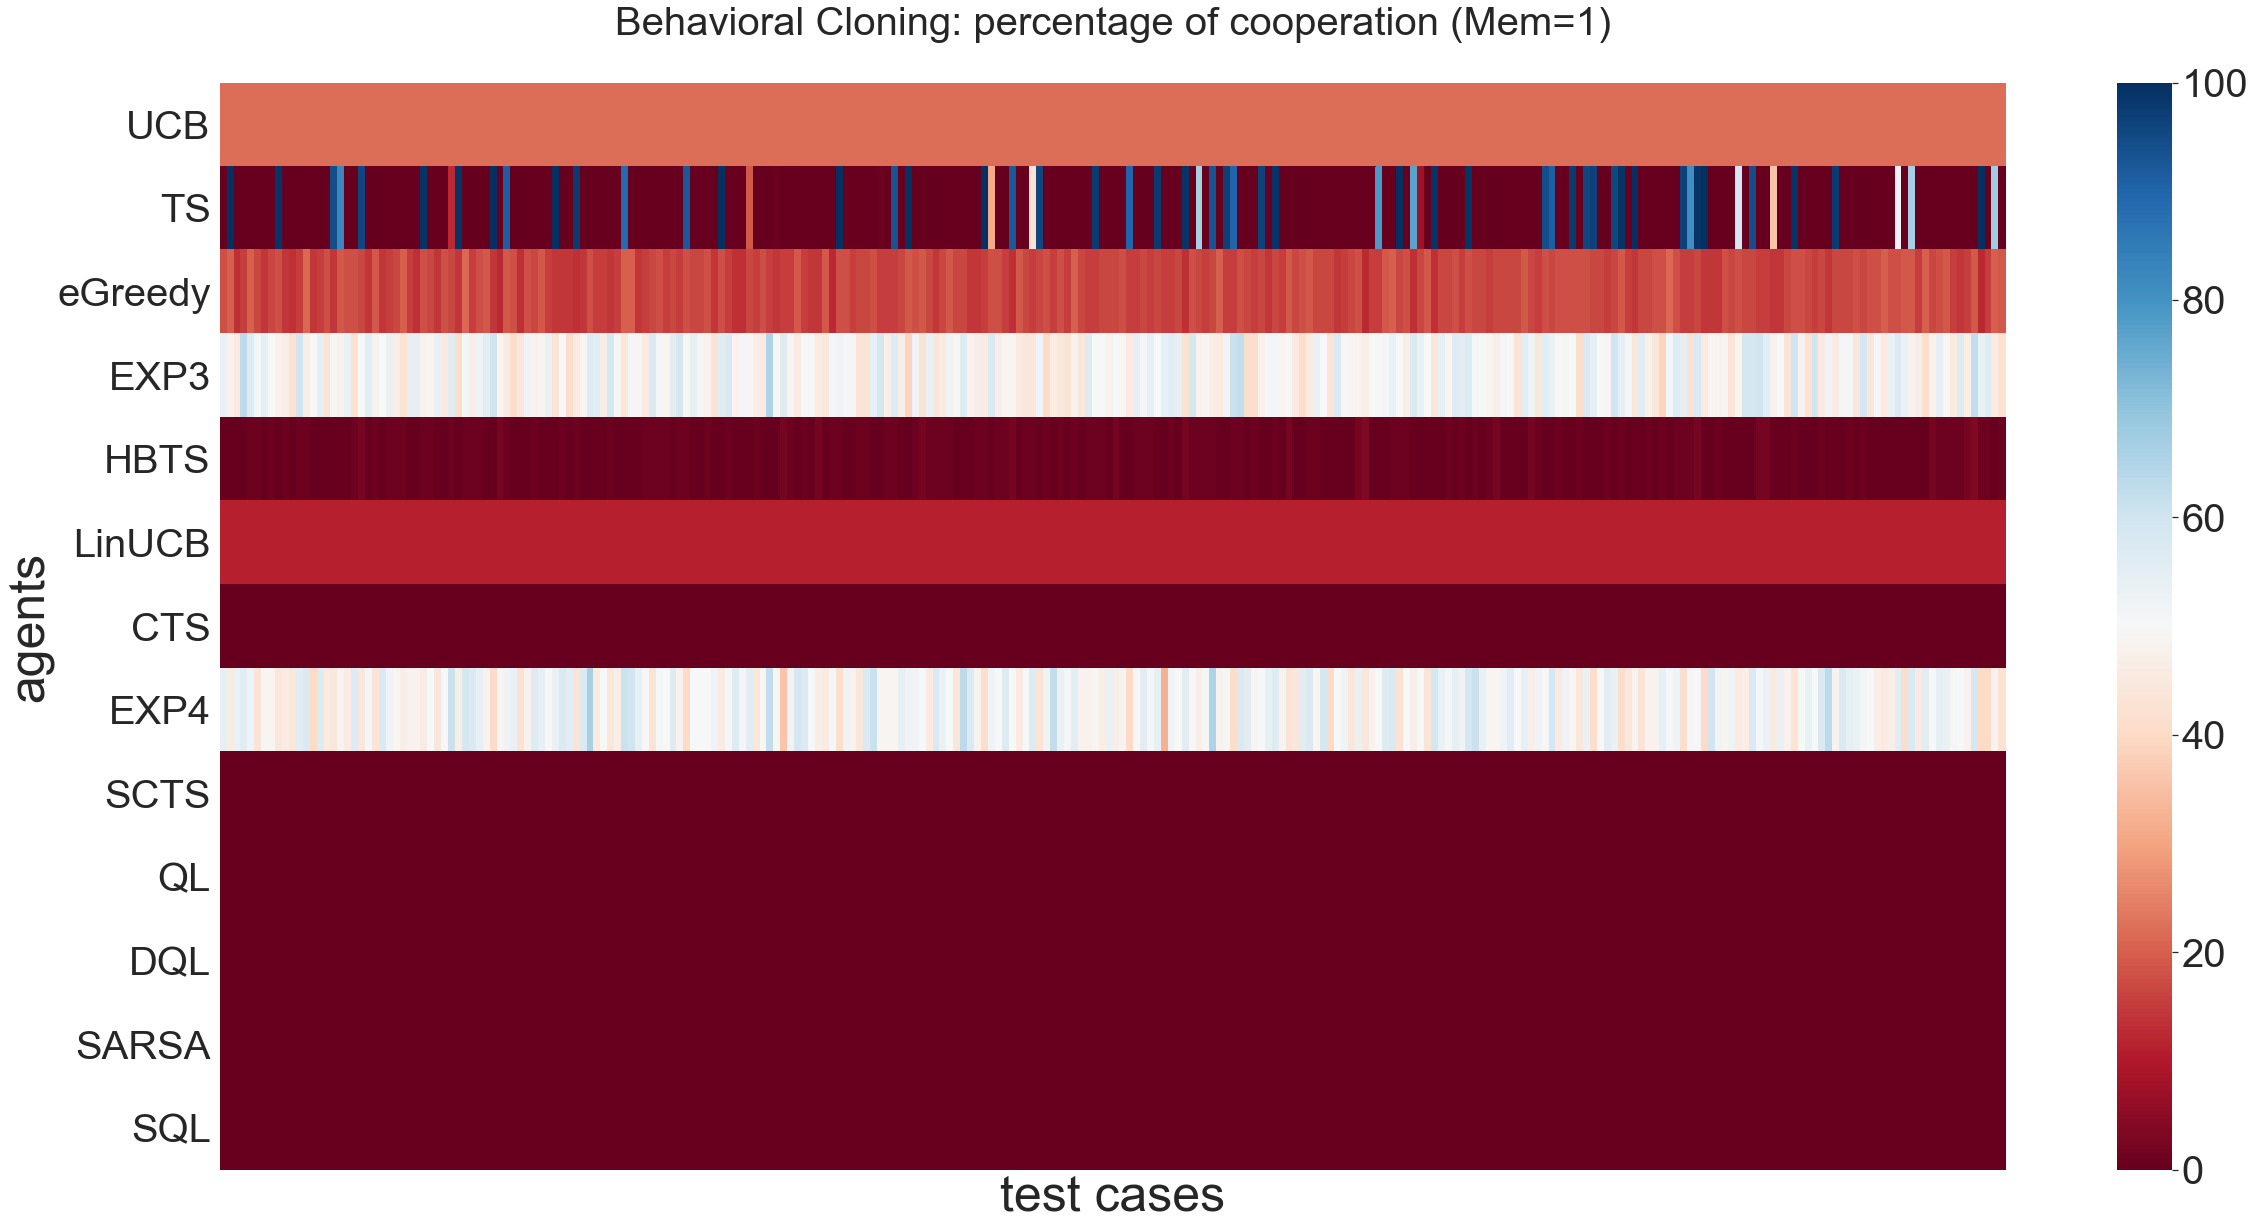}
\includegraphics[width=0.38\linewidth]{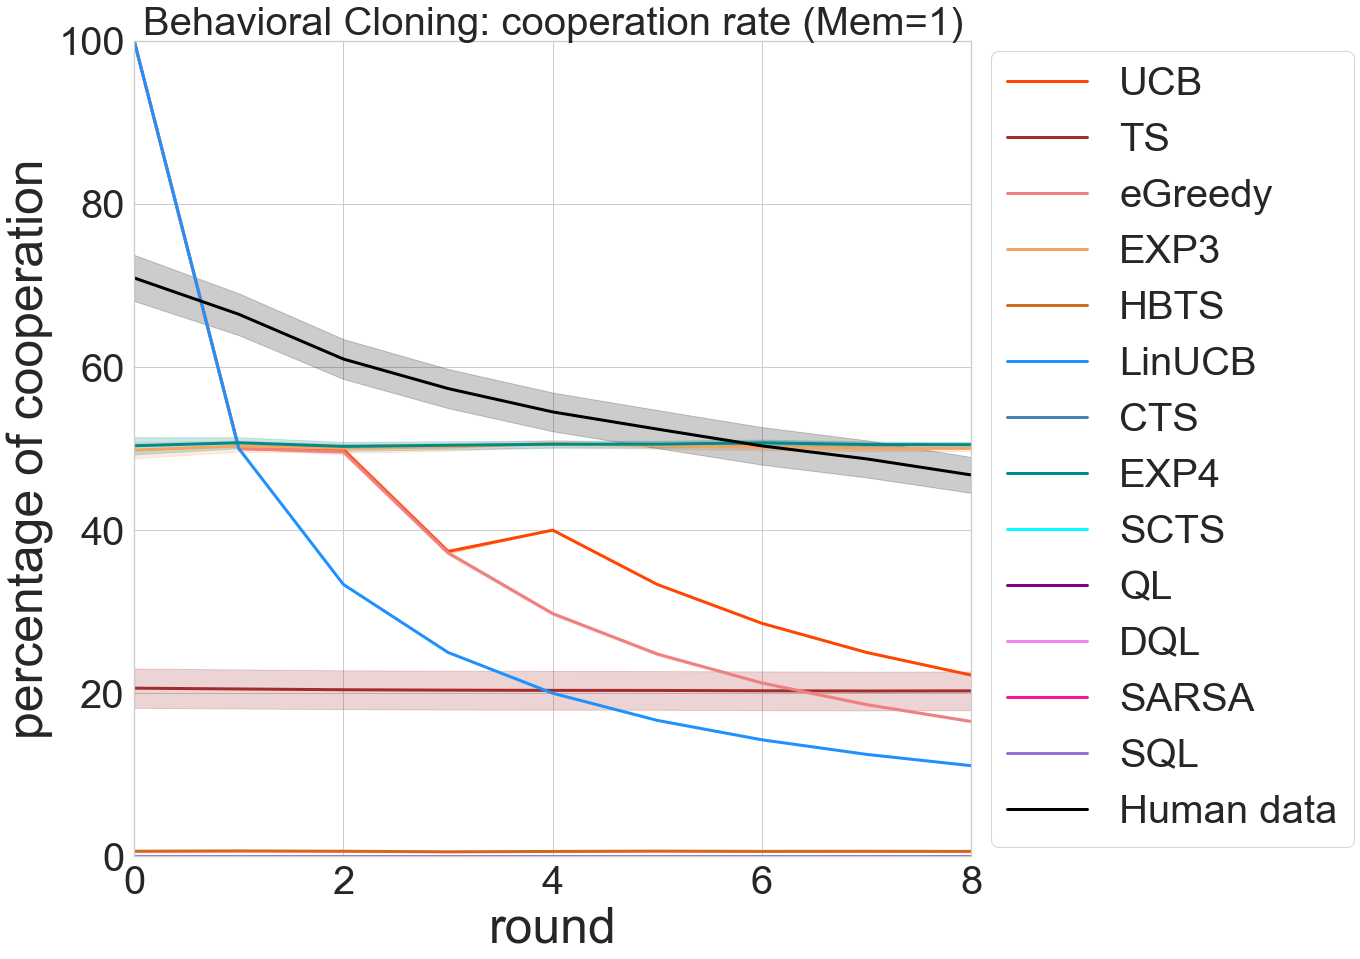}
\includegraphics[width=0.6\linewidth]{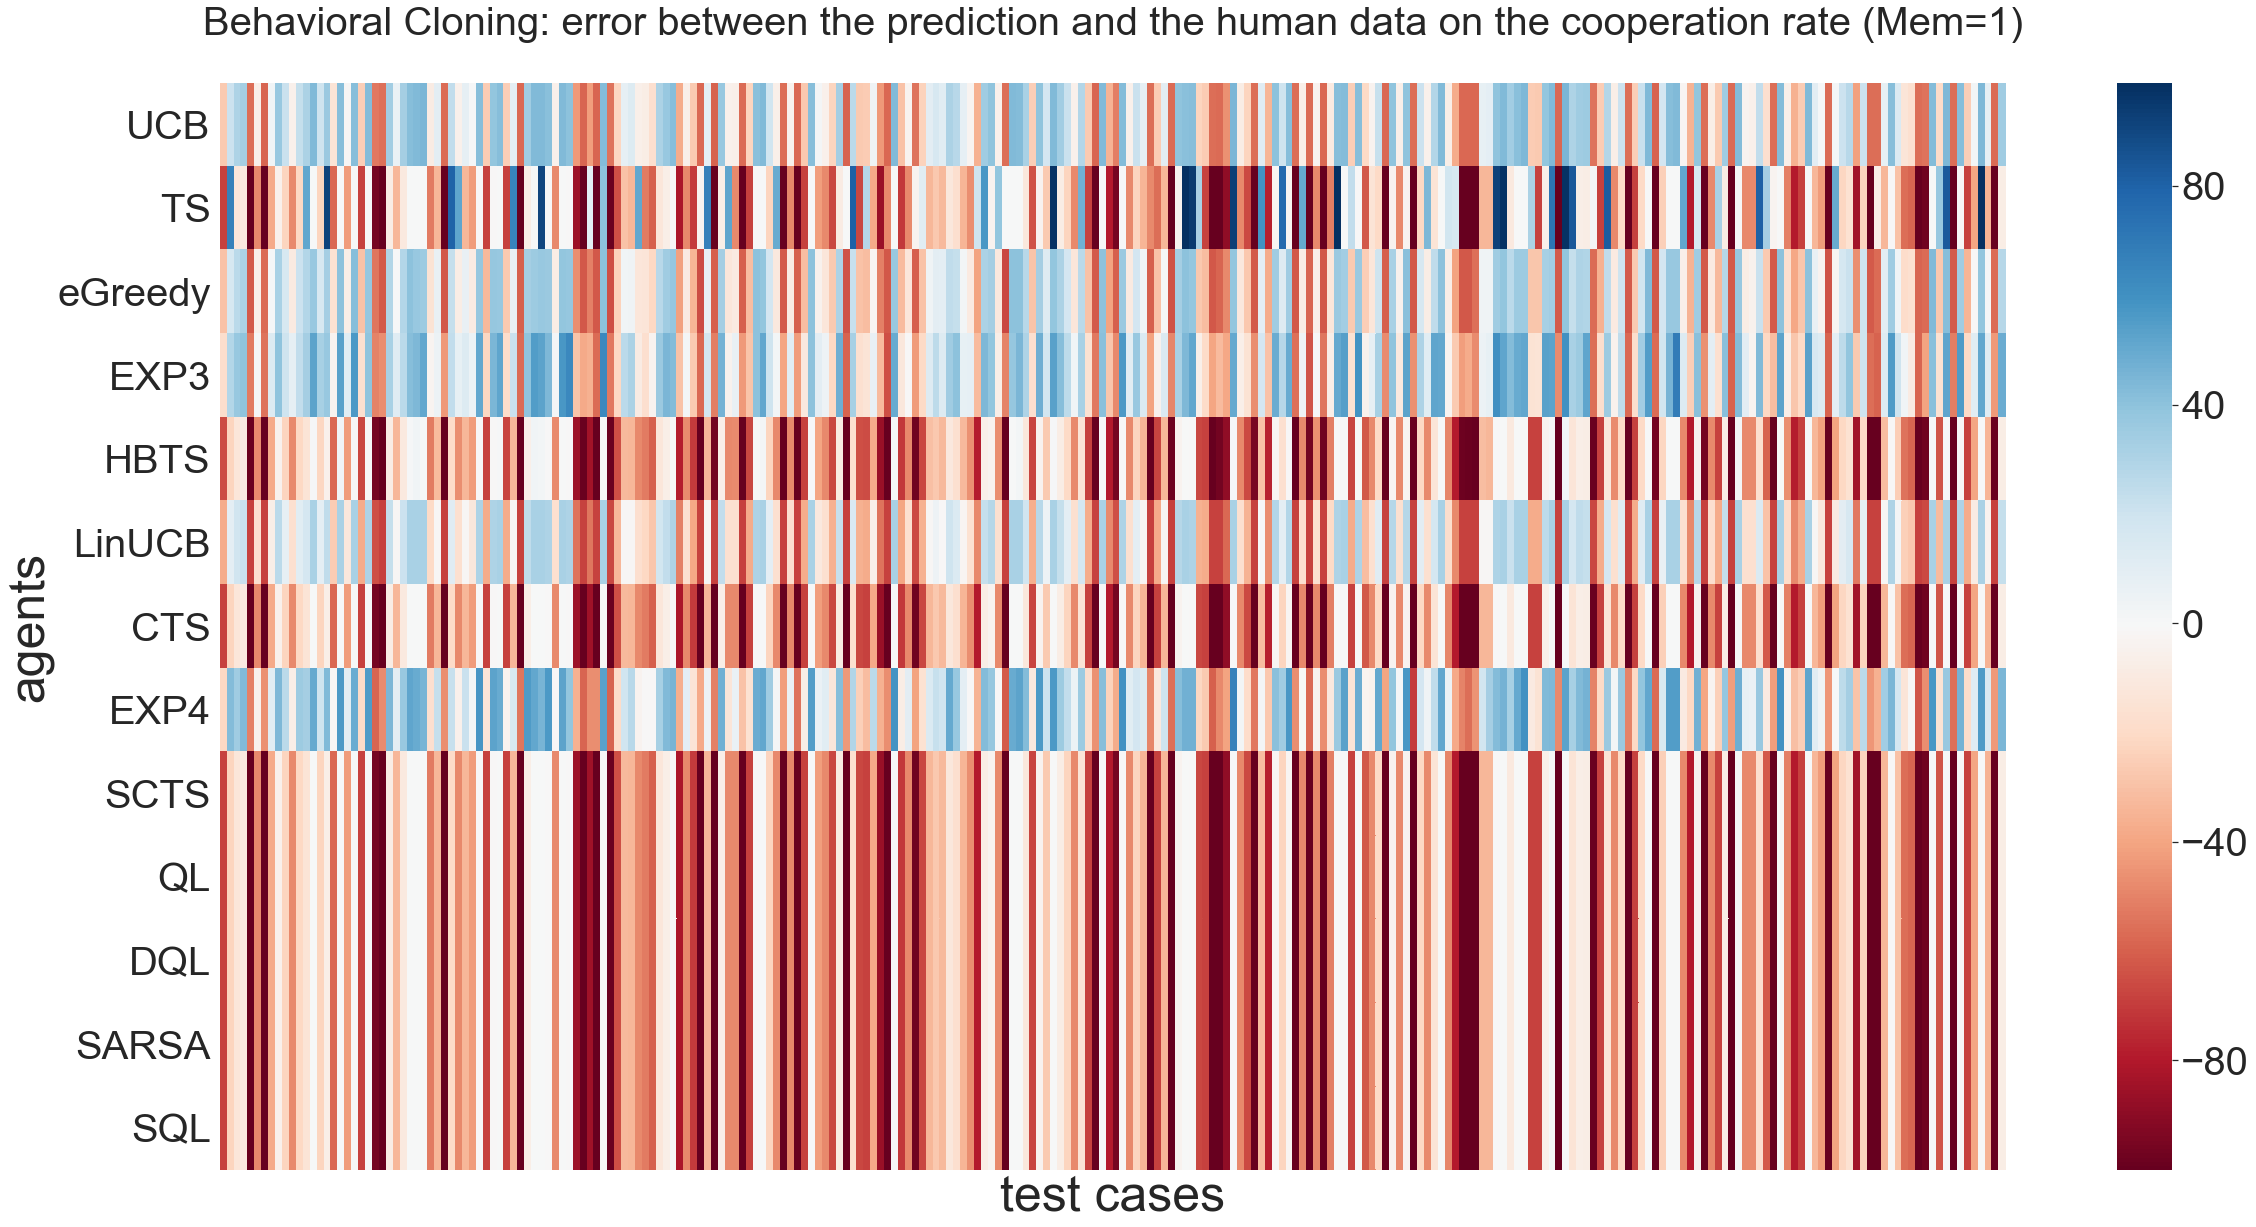}
\includegraphics[width=0.38\linewidth]{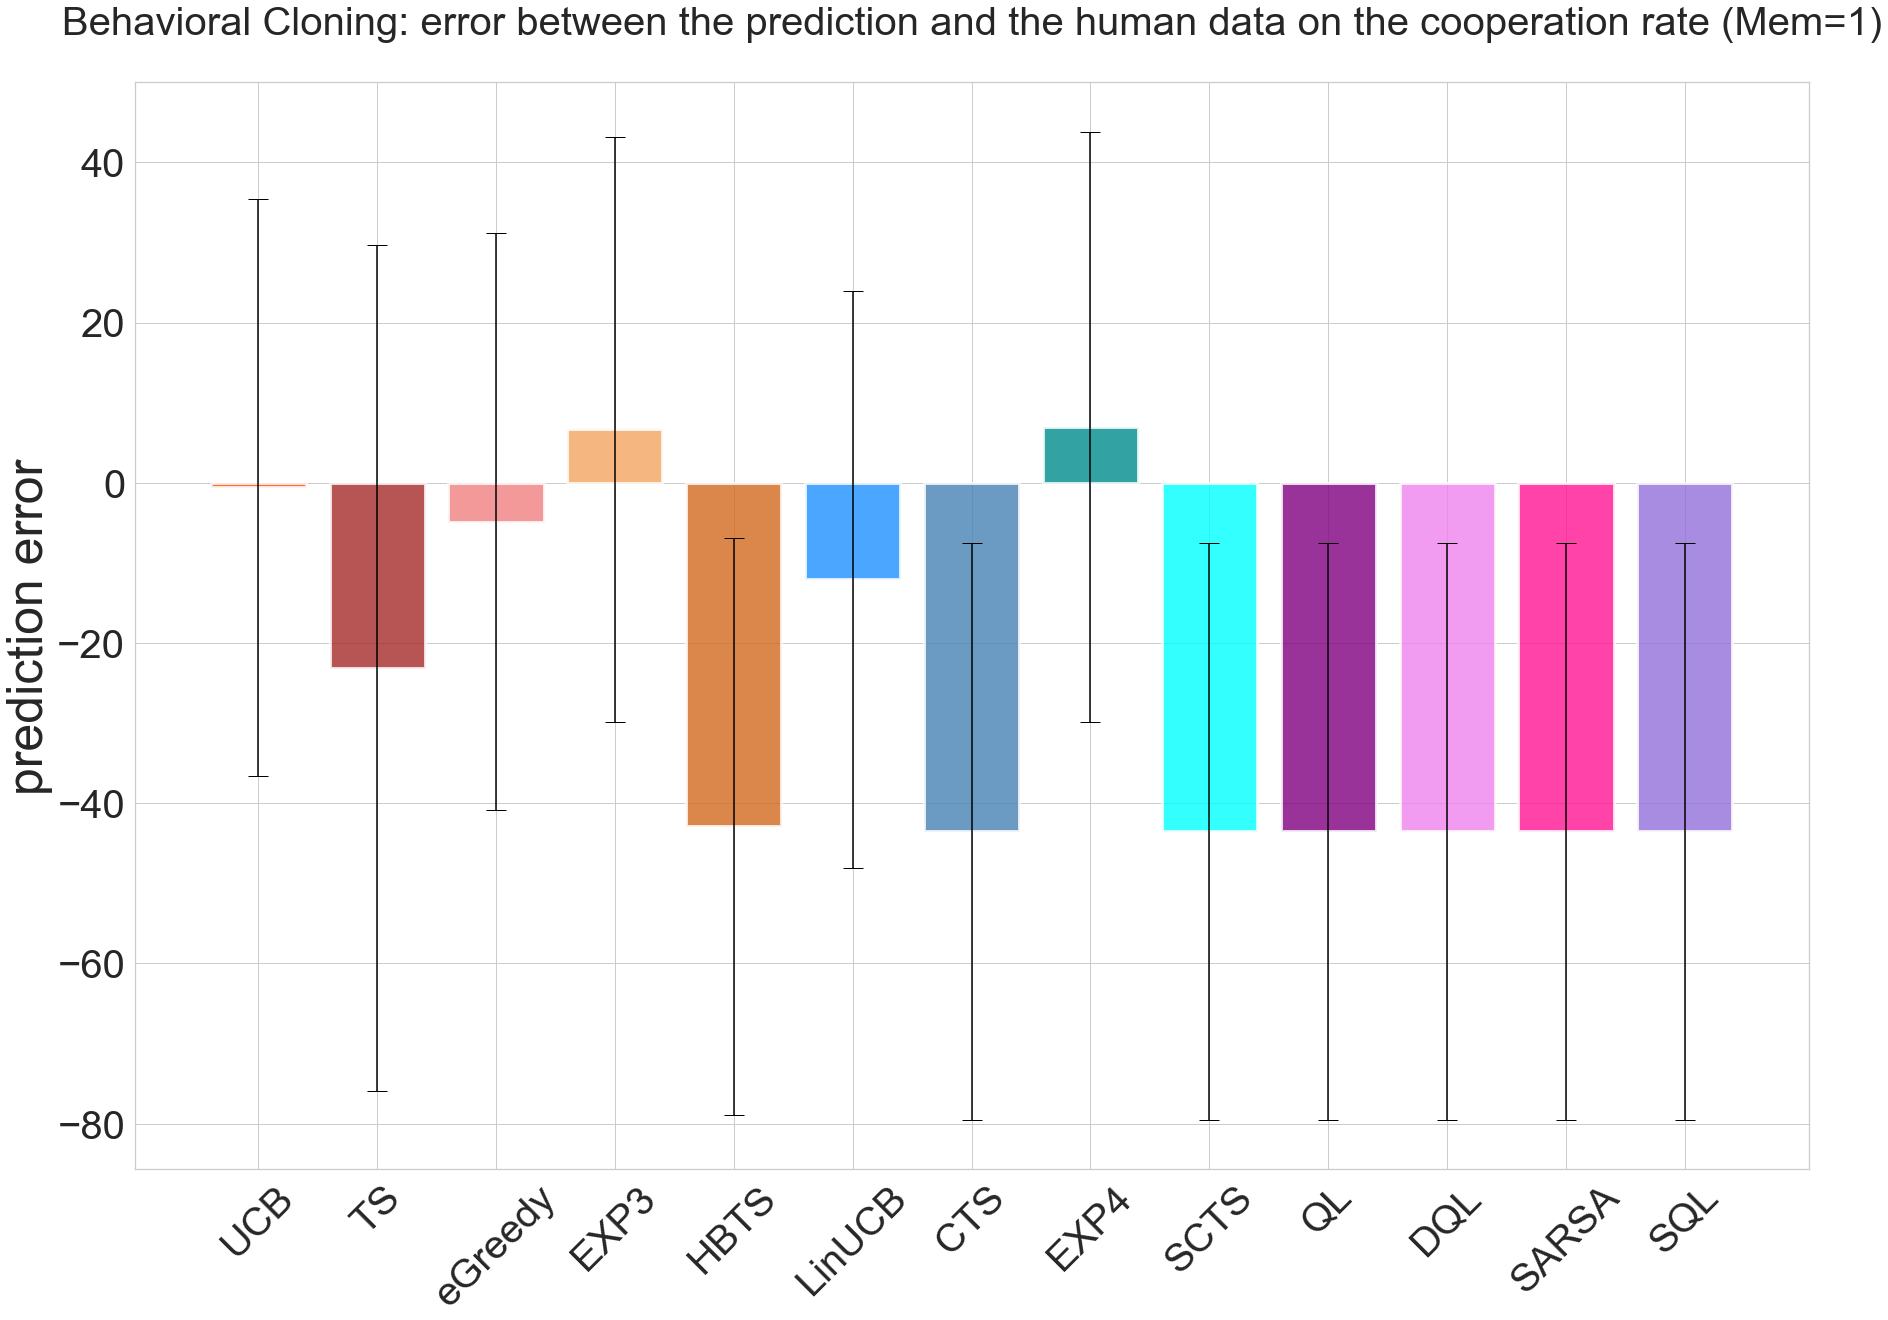}
\par\caption{Behavioral Cloning: bandit algorithms seem to better capture human data with lower prediction error (shown here the models trained with memory of 1 past action pairs).}\label{fig:bclone2}
\end{figure}
